# Supplementary material for: Computably Continuous Reinforcement-Learning Objectives are PAC-learnable
Source: arXiv:2303.05518 source file (2023-03-19)
Supplement: Supplementary file 2 [file aaai23-appendix-aux.tex]

\begin{filecontents}
{aaai23-appendix.aux}
\relax 
\bibstyle{aaai23}
\citation{dorsa14}
\citation{omegaregularrl19}
\citation{omegaregularrl19}
\citation{hasanbeig2019reinforcement}
\citation{omegaregularrl19}
\citation{dorsa14}
\citation{bozkurt2020control}
\citation{omegaregularrl20}
\citation{ltlnonpac22}
\newlabel{sec:summary-rl-automaton-objectives}{{A}{1}}
\newlabel{sec:summary-rl-automaton-objectives@cref}{{[appendix][1][]A}{[1][1][]1}}
\newlabel{sec:label_preserves_uniform_continuity_proof}{{B}{1}}
\newlabel{sec:label_preserves_uniform_continuity_proof@cref}{{[appendix][2][]B}{[1][1][]1}}
\newlabel{eq:proof_lemma3_eq1}{{B.1}{1}}
\newlabel{eq:proof_lemma3_eq1@cref}{{[equation][1][2]B.1}{[1][1][]1}}
\newlabel{eq:proof_lemma3_eq2}{{B.2}{1}}
\newlabel{eq:proof_lemma3_eq2@cref}{{[equation][2][2]B.2}{[1][1][]1}}
\newlabel{sec:computing-modulus-of-continuity}{{C}{1}}
\newlabel{sec:computing-modulus-of-continuity@cref}{{[appendix][3][]C}{[1][1][]1}}
\newlabel{lst:compute-modulus-of-continuity}{{C.1}{1}}
\newlabel{lst:compute-modulus-of-continuity@cref}{{[listing][1][3]C.1}{[1][1][]1}}
\providecommand*\caption@xref[2]{\@setref\relax\@undefined{#1}}
\newlabel{lst:rl-computable-objective}{{D.1}{2}}
\newlabel{lst:rl-computable-objective@cref}{{[listing][1][4]D.1}{[1][2][]2}}
\newlabel{sec:concrete-pac-rl-algorithm}{{D}{2}}
\newlabel{sec:concrete-pac-rl-algorithm@cref}{{[appendix][4][]D}{[1][1][]2}}
\newlabel{sec:proof-of-unnecessity}{{E}{2}}
\newlabel{sec:proof-of-unnecessity@cref}{{[appendix][5][]E}{[1][2][]2}}
\newlabel{sec:bozkurt_objective_pac_proof}{{F}{2}}
\newlabel{sec:bozkurt_objective_pac_proof@cref}{{[appendix][6][]F}{[1][2][]2}}
\citation{gltl17}
\newlabel{sec:gltl}{{G}{3}}
\newlabel{sec:gltl@cref}{{[appendix][7][]G}{[1][3][]3}}
\newlabel{eq:gnl_grammar}{{G.1}{3}}
\newlabel{eq:gnl_grammar@cref}{{[equation][1][7]G.1}{[1][3][]3}}
\newlabel{eq:gnl_event_interrupttrans}{{G.2}{3}}
\newlabel{eq:gnl_event_interrupttrans@cref}{{[equation][2][7]G.2}{[1][3][]3}}
\newlabel{eq:gltl_satisfaction_probability_function}{{G.3}{4}}
\newlabel{eq:gltl_satisfaction_probability_function@cref}{{[equation][3][7]G.3}{[1][4][]4}}
\newlabel{lemma:simu_expire}{{G.2}{4}}
\newlabel{lemma:simu_expire@cref}{{[lemma][2][7]G.2}{[1][4][]4}}
\newlabel{lemma:gltl-is-uc}{{G.3}{4}}
\newlabel{lemma:gltl-is-uc@cref}{{[lemma][3][7]G.3}{[1][4][]4}}
\newlabel{eq:gltl_satisfaction_probability_function-expand}{{G.5}{4}}
\newlabel{eq:gltl_satisfaction_probability_function-expand@cref}{{[equation][5][7]G.5}{[1][4][]4}}
\citation{principlesofmodelchecking}
\newlabel{lst:gltl-objective}{{G.1}{5}}
\newlabel{lst:gltl-objective@cref}{{[listing][1][7]G.1}{[1][5][]5}}
\newlabel{eq:gltl_satisfaction_probability_function-partial-sum}{{G.6}{5}}
\newlabel{eq:gltl_satisfaction_probability_function-partial-sum@cref}{{[equation][6][7]G.6}{[1][5][]5}}
\newlabel{sec:proof_simu_expire}{{H}{5}}
\newlabel{sec:proof_simu_expire@cref}{{[appendix][8][]H}{[1][5][]5}}
\newlabel{eq:gltl_lemma_g_eq1}{{H.1}{6}}
\newlabel{eq:gltl_lemma_g_eq1@cref}{{[equation][1][8]H.1}{[1][6][]6}}
\newlabel{eq:gltl_lemma_g_eq2}{{H.2}{6}}
\newlabel{eq:gltl_lemma_g_eq2@cref}{{[equation][2][8]H.2}{[1][6][]6}}
\newlabel{eq:gltl_lemma_g_eq3}{{H.3}{6}}
\newlabel{eq:gltl_lemma_g_eq3@cref}{{[equation][3][8]H.3}{[1][6][]6}}
\newlabel{eq:gltl_lemma_u_eq1}{{H.4}{6}}
\newlabel{eq:gltl_lemma_u_eq1@cref}{{[equation][4][8]H.4}{[1][6][]6}}
\newlabel{eq:gltl_lemma_u_eq2}{{H.5}{6}}
\newlabel{eq:gltl_lemma_u_eq2@cref}{{[equation][5][8]H.5}{[1][6][]6}}
\newlabel{eq:gltl_lemma_u_eq3}{{H.6}{6}}
\newlabel{eq:gltl_lemma_u_eq3@cref}{{[equation][6][8]H.6}{[1][6][]6}}
\citation{principlesofmodelchecking}
\bibdata{paper}
\bibcite{principlesofmodelchecking}{{1}{2008}{{Baier and Katoen}}{{}}}
\bibcite{bozkurt2020control}{{2}{2020}{{Bozkurt et~al.}}{{Bozkurt, Wang, Zavlanos, and Pajic}}}
\bibcite{omegaregularrl20}{{3}{2020}{{Hahn et~al.}}{{Hahn, Perez, Schewe, Somenzi, Trivedi, and Wojtczak}}}
\bibcite{omegaregularrl19}{{4}{2019}{{Hahn et~al.}}{{Hahn, Perez, Schewe, Somenzi, Trivedi, and Wojtczak}}}
\bibcite{hasanbeig2019reinforcement}{{5}{2019}{{Hasanbeig et~al.}}{{Hasanbeig, Kantaros, Abate, Kroening, Pappas, and Lee}}}
\bibcite{gltl17}{{6}{2017}{{Littman et~al.}}{{Littman, Topcu, Fu, Isbell, Wen, and MacGlashan}}}
\bibcite{dorsa14}{{7}{2014}{{Sadigh et~al.}}{{Sadigh, Kim, Coogan, Sastry, and Seshia}}}
\bibcite{ltlnonpac22}{{8}{2022}{{Yang, Littman, and Carbin}}{{}}}
\newlabel{sec:ltl_semantics}{{I}{7}}
\newlabel{sec:ltl_semantics@cref}{{[appendix][9][]I}{[1][7][]7}}
\newlabel{eq:ltl_grammar}{{I.1}{7}}
\newlabel{eq:ltl_grammar@cref}{{[equation][1][9]I.1}{[1][7][]7}}
\newlabel{eq:ltl_semantics}{{I.2}{7}}
\newlabel{eq:ltl_semantics@cref}{{[equation][2][9]I.2}{[1][7][]7}}
\gdef \@abspage@last{7}
\end{filecontents}
